# Supplementary material for: GenAIPABench: A Benchmark for Generative AI-based Privacy Assistants
Source: arXiv:2309.05138 source file (2023-12-19)
Supplement: Supplementary file 1 [file appendix_.tex]

% \begin{table*}[ht]
% \centering
% \begin{tabular}{|p{3cm}|p{10cm}|c|}
% \toprule
% \textbf{Category} & \textbf{Question}  & \textbf{Difficulty} \\
% \midrule
% \multirow{3}{=}{Transparency} & Does the policy avoid using technical phrases or legalese that might mislead users? & Easy \\
%  & What is the business' position on demands from the government for user data? & Medium \\
%  & How does the privacy policy manage any conflicts of interest with regard to the application or exchange of data? & Hard \\
% \midrule
% \multirow{3}{=}{User Control} & Do users have access to their data and privacy settings? &  Easy \\
%  & Are there straightforward methods for users to request data access or deletion? & Medium \\
%  & How does the business handle user approval and revocation of approval? & Hard \\
% \midrule
% \multirow{3}{=}{Data Minimization and Purpose Limitation} & Does the business reduce storage times? & Easy \\
%  & How is user data aggregated or masked to safeguard personal information? & Medium \\
%  & Are there any limitations on how data may be processed for particular situations or purposes? & Hard \\
% \midrule
% \multirow{3}{=}{Security and Encryption} & Do user communications employ end-to-end encryption? & Easy \\
%  & How are user data being accessed without authorization prevented? & Medium \\
%  & How are security-related incidents or thefts of information handled and informed to users? & Hard \\
% \midrule
% \multirow{3}{=}{Privacy by Design and Innovation} & Does the organization carry out privacy impact analyses? & Easy \\
%  & Have any privacy-enhancing technologies, such as differential privacy, been implemented? & Medium \\
%  & How does the use of automated decision-making or profiling by the firm affect the privacy of its customers? & Hard \\
% \midrule
% \multirow{3}{=}{Responsiveness and Communication} & Is the privacy policy updated frequently and made available to users? & Easy \\
%  & Does a procedure exist to handle user privacy complaints? & Medium \\
%  & Does the business release transparency reports describing interactions with law enforcement or government agencies or data requests for surveillance? & Hard \\
% \midrule
% \multirow{3}{=}{Accessibility, User Education and Empowerment} & Do employees receive training on handling sensitive information and best practices for data privacy? & Easy \\
%  & How are user choices for data privacy maintained across many platforms or devices? & Medium \\
%  & Does the company provide easy-to-use resources, such as tutorials or guides, to help users successfully manage their privacy settings and comprehend their data rights? & Hard \\
% \midrule
% \multirow{3}{=}{Compliance and Accountability} & Does this policy conform with all relevant privacy laws and regulations? & Easy \\
%  & What measures are made to guarantee that data processors and subprocessors respect privacy standards? & Medium \\
%  & Is there a procedure in place at the business for reporting and dealing with privacy violations or non-compliance issues, both internally and with third-party vendors? & Hard \\
% \bottomrule
% \end{tabular}
% \caption{Paraphrased privacy policy questions.}
% \label{fig:para}
% \end{table*}
